# Supplementary material for: Make-Your-Anchor: A Diffusion-based 2D Avatar Generation Framework
Source: arXiv:2403.16510 source file (2024-03-25)
Supplement: Supplementary file 1 [file X_suppl.tex]

%\clearpage
\setcounter{page}{1}
\setcounter{section}{0}
\setcounter{table}{0}
\setcounter{figure}{0}

\maketitlesupplementary

\section{Related Work}
\label{sec:related_work}
\subsection{Talking Face Generation}
Talking face generation methods~\cite{prajwal2020wav2lip, zhang2023sadtalker, cheng2022videoretalking, wang2021facevid2vid} generate human videos with various expressions and poses conditioned on a given audio or motion, which can be categorized into two types: editing facial regions or generating dynamic head videos.
Editing-based techniques, such as Wav2Lip~\cite{prajwal2020wav2lip} or VideoRetalking~\cite{cheng2022videoretalking}, face the problem of lip-gesture inconsistency.
Usually, the gestures are fixed for different talking content.
Generating dynamic head video requires methods to create head videos conditioned on given audio or motion, where head motions are accomplished by different manners such as motion flow~\cite{yin2022styleheat}, 3D landmarks~\cite{wang2021facevid2vid, zhang2023sadtalker}, self-supervised training~\cite{pang2023dpe}, etc.
Although producing high-quality and highly realistic facial videos, talking face generation is limited by its interest area and cannot achieve full-body human video generation.
 
\subsection{Pose-guided Human Video Generation}
To generate human video with body and hand, pose-guided methods are the most popular approaches.
Early work focuses on the problem of motion transfer~\cite{motiontransfer_balakrishnan2018warpingbyICCV2021, motiontransfer_chan2019everybodydance, motiontransfer_siarohin2019fomm, motiontransfer_liu2019liquidwarpinggan, motiontransfer_siarohin2021mraa, motiontransfer_zhao2022tpsmotion, motiontransfer_siarohin2023unsupervised, motiontransfer_wang2022lia, motiontransfer_yang2022delving} methods.
Balakrishnan et al.~\cite{motiontransfer_balakrishnan2018warpingbyICCV2021} separate a scene and transform each part to synthesize.
% Chan et al.~\cite{motiontransfer_chan2019everybodydance} utilize pretrained pose to represent the body and transfer the appearance of the identity in the training dataset.
% Liu et al.~\cite{motiontransfer_liu2019liquidwarpinggan} decouple the task into mesh recovery, flow composition, and warping.
FOMM~\cite{motiontransfer_siarohin2019fomm} and MRAA~\cite{motiontransfer_siarohin2021mraa} propose unsupervised body representation and warping to transfer, while LIA~\cite{motiontransfer_wang2022lia} employs latent space.
TPS~\cite{motiontransfer_zhao2022tpsmotion} introduces thin plate spline transformation into a motion transfer task, and UVA~\cite{motiontransfer_siarohin2023unsupervised} presents a differential volumetric representation.
Besides the coarse-grained motion transfer setting, researchers~\cite{cogesture_ginosar2019learningstylegesture, cogesture_qian2021speechdrivetemplates, cogesture_zhou2022audiodriven-videomotiongraphs, cogesture_liao2020speech2video} apply these kinds of methods into human video generation with face, body, and hand.
However, constrained to the capability of these models, these methods potentially generate human videos with apparent artifacts.

With the progress of diffusion models~\cite{ho2020ddpm, rombach2022ldm}, some works introduce them into pose-guided human video generation.
Follow-your-pose~\cite{ma2023followyourpose} introduces a two-stage training to get a pose-guided video diffusion model.
DreamPose~\cite{karras2023dreampose} proposes a vision and pose controlled diffusion on fashion dataset to animate a body image.
DisCo~\cite{wang2023disco} focuses on human dance generation, utilizes multiple ControlNet on pose and background, and introduces a pretraining strategy to improve generalizability.
Nonetheless, these methods concentrate on coarse-grained body video generation, which is limited to the poor quality of face and hands. 
Besides, due to the randomness of the diffusion model, these methods struggle with temporal consistency.
The proposed system, by proposing a simple yet efficient multi-frame inference strategy, could improve the temporal consistency of image-based diffusion models.
%\ziyao{MagicAvatar~\cite{zhang2023magicavatar} is the most relevant work with ours, which supports avatar animation from multiple motion inputs (e.g., human pose, depth, DensePose), however, it is still unsubstantiated of the ability to generate talking lips.}

\subsection{Video Diffusion Models}
Due to the powerful capabilities of diffusion models, researchers in recent years have started to explore their potential in video generation, and much progress has been made in video generation~\cite{ho2022imagenvideo, singer2022makeavideo, blattmann2023alignyourlatents, chen2023videocrafter1, ge2023preserveyourcorrelation} and video editing~\cite{chai2023stablevideo, QI_2023fatezero, yang2023rerender}.
GEN-1~\cite{esser2023gen1} extends the image diffusion model with a temporal module and utilizes depth to control the structure.
Tune-A-Video~\cite{Wu_2023_tuneavideo} fine-tunes 3D U-Net in image diffusion model on a one-shot video to learn the motion and then edits the video content with text prompts.
AnimateDiff~\cite{guo2023animatediff} trains a temporal module with a fixed image diffusion model and can be applied to personalized weights.
% controlvideo, animatediff
While VDMs possess strong video generation capabilities, the ability to control human motion and maintain appearance needs further improvement.
In contrast, we tune the foundation diffusion model to learn the mapping from motion to a specific anchor appearance in a ``binding'' fashion following a pretrain-finetuning paradigm.
%and VDMs cannot be directly used for synthesizing human videos.\ziyao{not exactly}

%\subsection{Human Nerf}

\section{Video Results}
We show video results in the attached materials.
In the video, we compare with SOTA methods as well as present the results of ablation studies.
Video results demonstrate the effectiveness of the proposed method.
For example, we could observe slight flicking frames in the video results without overlapped batches.
This is due to the absence of information transfer between different batches and the inherent randomness of the diffusion model, resulting in subtle variations in human structure across batches.
The proposed overlapped-batch design in the denoising process allows for certain context exchanges between different batches, thereby reducing the occurrence of this phenomenon.

Furthermore, we show the results of audio-driven digital avatar generation. We utilize TalkSHOW~\cite{yi2023talkshow} to drive the 3D human mesh, and the examples are shown in the video as well as Fig.~\ref{fig:sup.audio_driven}.
By combining our method with existing audio-driven motion generation techniques, we create a system capable of automatically generating 2D avatar videos.

\begin{figure}[htp]
\newcommand{\galleryfigurewidth}{0.30}
\centering
    %%%%
    \begin{minipage}[t]{\linewidth}
    \centering
        \begin{minipage}{\galleryfigurewidth\linewidth}
            \includegraphics[width=\linewidth]{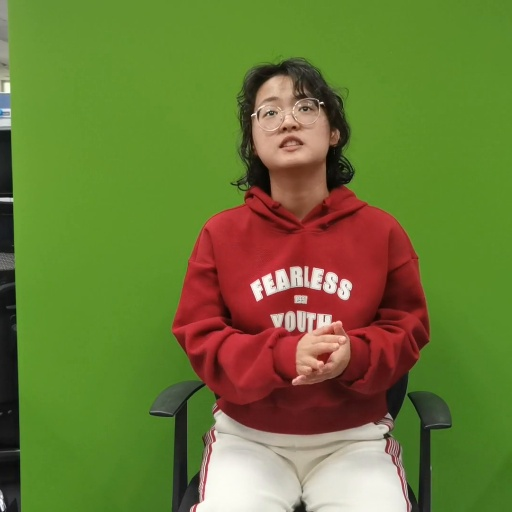}
            \includegraphics[width=\linewidth]{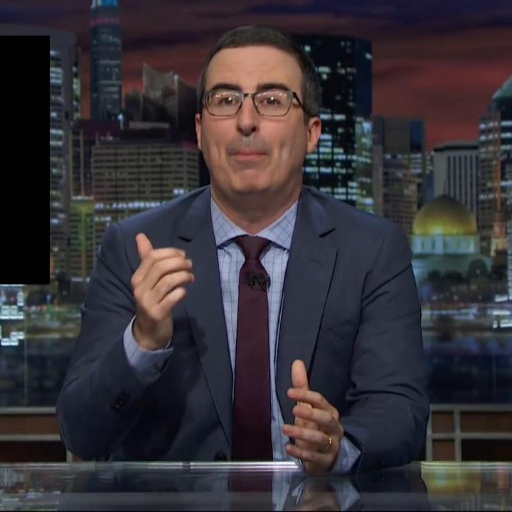}
        \end{minipage}
        \begin{minipage}{\galleryfigurewidth\linewidth}
            \includegraphics[width=\linewidth]{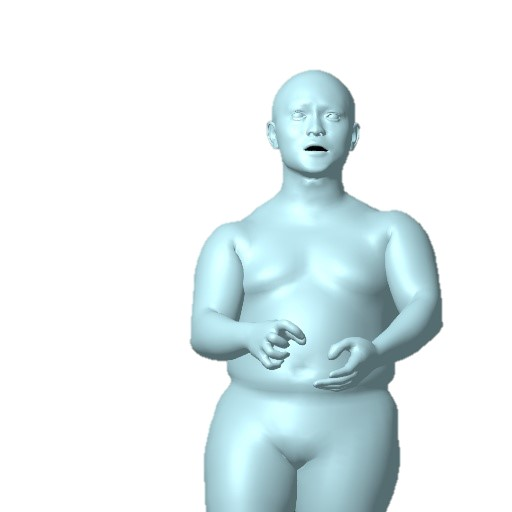}
            \includegraphics[width=\linewidth]{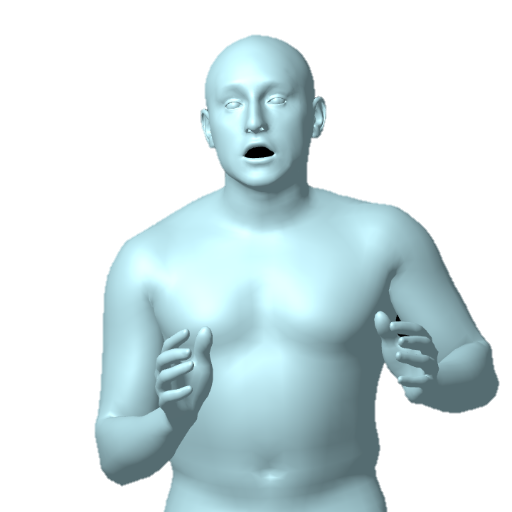}
        \end{minipage}
        \begin{minipage}{\galleryfigurewidth\linewidth}
            \includegraphics[width=\linewidth]{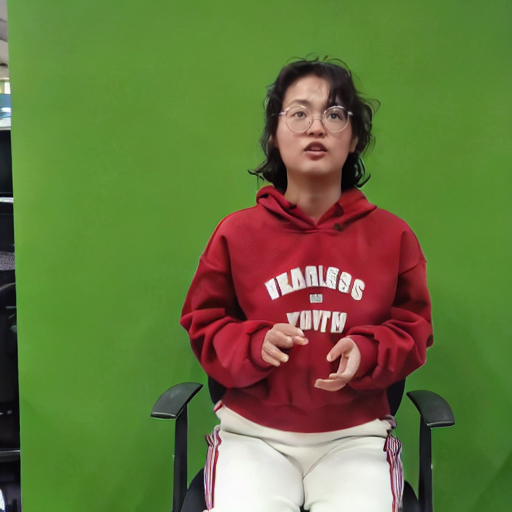}
            \includegraphics[width=\linewidth]{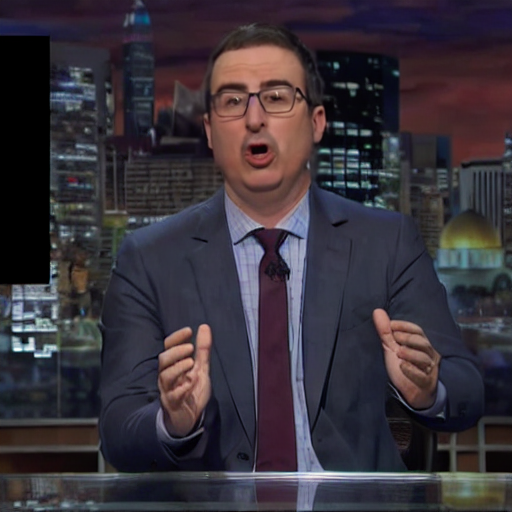}
        \end{minipage}

    \end{minipage}
\begin{subfigure}[t]{\galleryfigurewidth\linewidth}
    \subcaption*{Appearance}
\end{subfigure}
\begin{subfigure}[t]{\galleryfigurewidth\linewidth}
    \subcaption*{Audio-driven pose}
\end{subfigure}
\begin{subfigure}[t]{\galleryfigurewidth\linewidth}
    \subcaption*{Output}
\end{subfigure}
\caption{
Examples of audio-driven results.
}
\label{fig:sup.audio_driven}
\end{figure}

\section{User Study}

We conduct user studies under our experimental setting in the main text.
The videos generated in Section 5.2 were collected, and we invited $30$ participants to operate this user study.
For each participant, $15$ video instances are randomly sampled from all results, and the corresponding reference appearance and input pose sequence are shown simultaneously.
For each instance, we asked participants to rate from four aspects: appearance preservation, temporal consistency, structure preservation, and overall quality.
Appearance preservation measures the appearance between the reference image and the generated video.
Structure preservation is asked to evaluate the structure similarity between input pose and output video, especially for hand structure.
The rating score of each question is on a scale from one to five, with five being the highest score and one being the lowest.

The statistics are listed in Table~\ref{tab:userstudy}.
As the results show, our method achieves the best scores of over four points in the user study.
Pose2Img scored above three points in appearance preservation, and the results from Dreampose and DisCo are slightly inferior to Pose2Img.
Our method has achieved a significant advantage in structure preservation compared to other methods, which is not apparent by LMD in Table 1 of the main text for inaccurately estimated landmarks.
\begin{table}[!h]
  \centering
  \resizebox{\linewidth}{!}{
  \begin{tabular}{@{}lcccc@{}}
    \toprule
    \multirow{2}{*}{Method}                                               & Appearance        & Temporal      & Structure             & Overall           \\
                                                                          &  Preservation     & Consistency   & Preservation          & Quality           \\
    \midrule
    Pose2Img~\cite{cogesture_qian2021speechdrivetemplates}                & 3.36              & 2.38          & 1.59                  & 2.01              \\
    TPS~\cite{motiontransfer_zhao2022tpsmotion}                           & 2.03              & 2.10          & 1.18                  & 1.37              \\
    DreamPose~\cite{karras2023dreampose}                                  & 2.78              & 1.94          & 2.27                  & 1.94              \\
    DisCo~\cite{wang2023disco}                                            & 2.29              & 2.32          & 1.45                  & 1.72              \\
    Ours                                                                  & \textbf{4.23}     & \textbf{3.85} & \textbf{3.91}         & \textbf{4.03}     \\
    \bottomrule
  \end{tabular}}
  \caption{User study scores. The rating score is on a scale from one to five, where five is the highest score, and one is the lowest.}
  \label{tab:userstudy}
\end{table}

% BAK:

% \begin{table}[!h]
%   \centering
%   \resizebox{\linewidth}{!}{
%   \begin{tabular}{@{}lcccc@{}}
%     \toprule
%     \multirow{2}{*}{Method} & Appearance        & Temporal      & Structure             & Overall           \\
%                             &  Preservation     & Consistency   & Preservation          & Quality           \\
%     \midrule
%     Pose2Img                & 3.36              & 2.38          & 1.59                  & 2.01              \\
%     TPS                     & 2.03              & 2.10          & 1.18                  & 1.37              \\
%     DreamPose               & 2.78              & 1.94          & 2.27                  & 1.94              \\
%     DisCo                   & 2.27              & 2.32          & 1.45                  & 1.72              \\
%     Ours                    & \textbf{4.43}     & \textbf{4.21} & \textbf{4.05}         & \textbf{4.17}     \\
%     \bottomrule
%   \end{tabular}}
%   \caption{User study scores. The rating score is on a scale from one to five, where five is the highest score, and one is the lowest.}
%   \label{tab:userstudy}
% \end{table}

\section{Ablation on Video Length}
\label{sec:videolength}
We conducted an analysis of the required duration for video data needed for fine-tuning.
Compared to the one-minute videos used in the main text, we utilize five-minute videos in the fine-tuning stage.
The quantitative results are demonstrated in Table.~\ref{tab:ablation_videotime} and the qualitative results are displayed in Fig.~\ref{fig:ablation.videolength}.
The numerical results demonstrate a slight improvement in all measurements. 
For instance, with LMD (hand), additional data allows the model to encompass a broader range of angles, enabling more accurate generation outcomes, and showing better results.
In qualitative results, one minute of fine-tuning data already yields satisfactory outcomes.
\begin{figure}[htp]
\newcommand{\galleryfigurewidth}{0.24}
\centering
\begin{subfigure}[t]{\galleryfigurewidth\linewidth}
    \subcaption*{Frame1}
\end{subfigure}
\begin{subfigure}[t]{\galleryfigurewidth\linewidth}
    \subcaption*{Frame2}
\end{subfigure}
\begin{subfigure}[t]{\galleryfigurewidth\linewidth}
    \subcaption*{Frame3}
\end{subfigure}
\begin{subfigure}[t]{\galleryfigurewidth\linewidth}
    \subcaption*{Frame4}
\end{subfigure}
    \begin{minipage}[t]{\linewidth}
    \centering
        \begin{minipage}{\galleryfigurewidth\linewidth}
            \includegraphics[width=\linewidth]{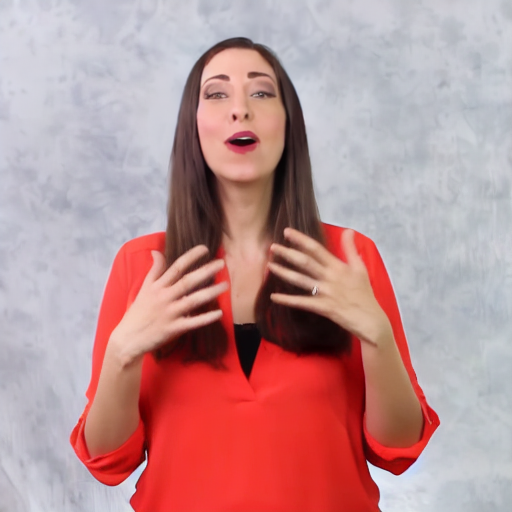}
        \end{minipage}
        \begin{minipage}{\galleryfigurewidth\linewidth}
            \includegraphics[width=\linewidth]{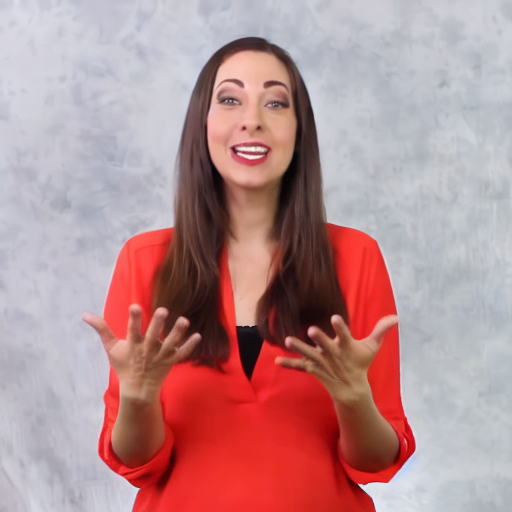}
        \end{minipage}
        \begin{minipage}{\galleryfigurewidth\linewidth}
            \includegraphics[width=\linewidth]{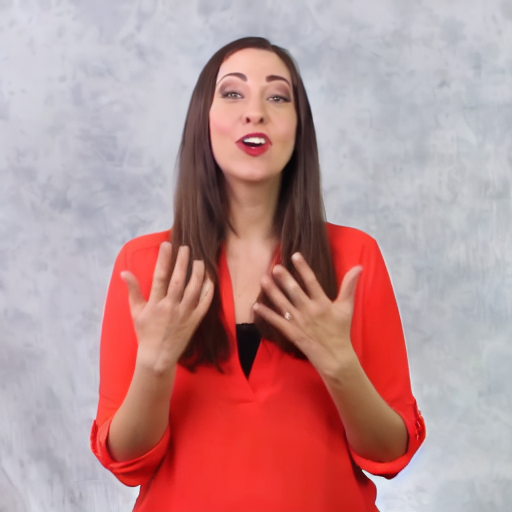}
        \end{minipage}
        \begin{minipage}{\galleryfigurewidth\linewidth}
            \includegraphics[width=\linewidth]{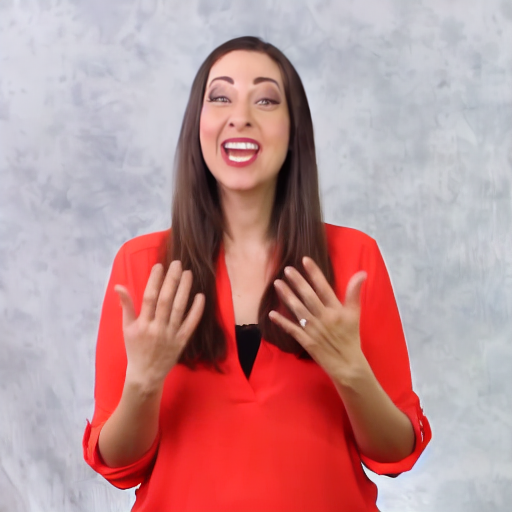}
        \end{minipage}
        \subcaption{Fine-tuning with one-minute videos}
    \end{minipage}

  \begin{minipage}[t]{\linewidth}
    \centering
        \begin{minipage}{\galleryfigurewidth\linewidth}
            \includegraphics[width=\linewidth]{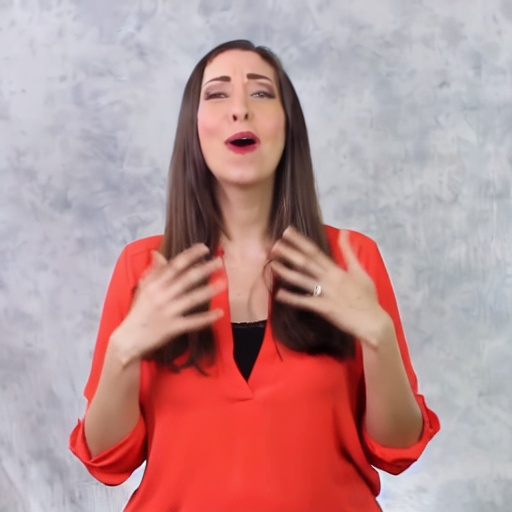}
        \end{minipage}
        \begin{minipage}{\galleryfigurewidth\linewidth}
            \includegraphics[width=\linewidth]{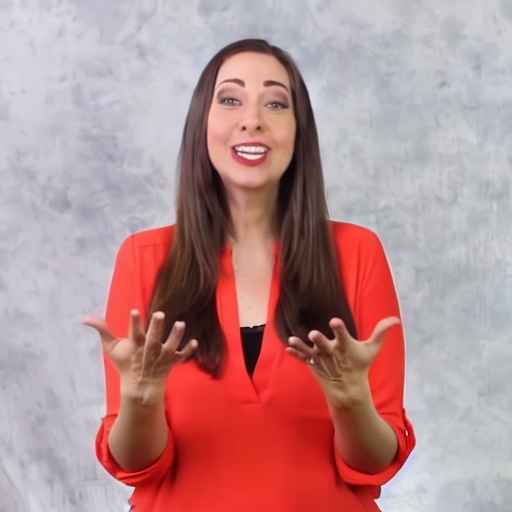}
        \end{minipage}
        \begin{minipage}{\galleryfigurewidth\linewidth}
            \includegraphics[width=\linewidth]{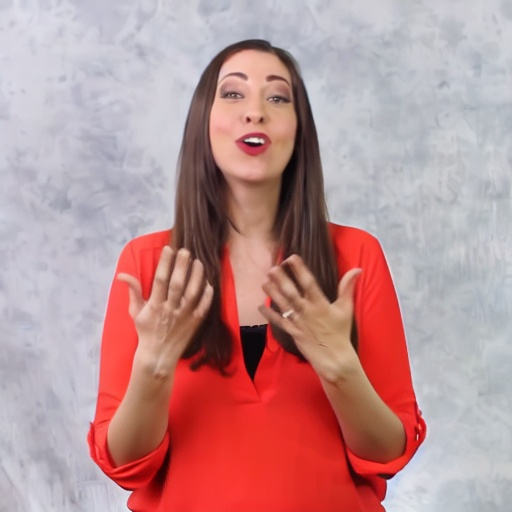}
        \end{minipage}
        \begin{minipage}{\galleryfigurewidth\linewidth}
            \includegraphics[width=\linewidth]{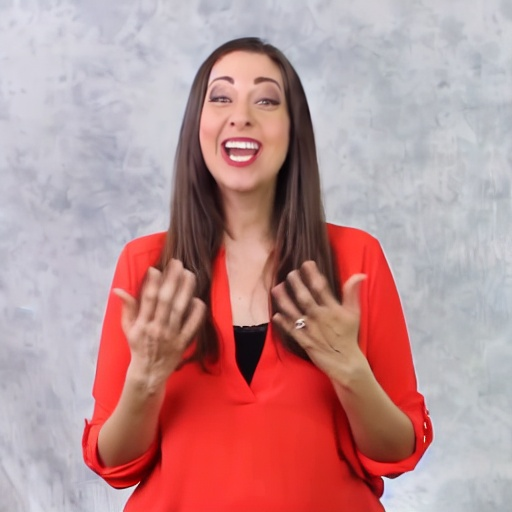}
        \end{minipage}
        \subcaption{Fine-tuning with five-minute videos}
    \end{minipage}

\caption{
  Qualitative results with different video lengths for fine-tuning.
}
\label{fig:ablation.videolength}
\end{figure}

\begin{table}[!ht]
  \centering
  \resizebox{\linewidth}{!}{
  \begin{tabular}{@{}lcccccc@{}}
    \toprule
    Fine-tuning with          & FID↓              & FVD↓           &    LMD (Face)↓    & LMD (Body)↓   & LMD (Hand)↓               \\
    \midrule
    One-minute videos         &  40.33            & 139.82         &    1.44           & 4.88          &  5.41    \\
    Five-minute videos        &  38.94            & 134.55         &    1.29           & 4.42          &  4.95     \\
    \bottomrule
  \end{tabular}
  }
  \caption{Ablation analysis of video length used for fine-tuning.}
  \label{tab:ablation_videotime}
\end{table}

% back
% \begin{table}[!ht]
%   \centering
%   \resizebox{\linewidth}{!}{
%   \begin{tabular}{@{}lcccccc@{}}
%     \toprule
%     Fine-tuning with                              & FID↓              &  FID-VID↓       & FVD↓           &    LMD (Face)↓    & LMD (Body)↓   & LMD (Hand)↓               \\
%     \midrule
%     One-minute videos         &  40.33            &  15.95          & 139.82         &    1.44           & 4.88          &  5.41    \\
%     Five-minute videos        &  38.94            &  15.45          & 134.55         &    1.29           & 4.42          &  4.95     \\
%     \bottomrule
%   \end{tabular}
%   }
%   \caption{Ablation analysis of video length used for fine-tuning.}
%   \label{tab:ablation_videotime}
% \end{table}

\section{Additional Time Cost.}
Time cost of different methods is shown in Table~\ref{tab:ablation.timecost}. Our method is comparable to other diffusion methods. Most time is spent on diffusion. Off-the-shelf speed-up approaches such as LCM~\cite{luo2023lcm} could be further engaged.

In Algorithm~1, $count$ is an array storing the computing counts for each frame, where only overlapped frames are calculated twice times.
When the $ws=16$ and $os=4$ for 300 frames/10s to generate, the total computing times in $count$ is 400, which means an additional one-third of the cost.
The additional time cost brings consistency between batches to generate long duration.
A comparison of time cost and ablation without batch-overlapped temporal denoising (TD) is listed in Table.~\ref{tab:ablation.timecost}.

\begin{table}
  \centering
  \resizebox{\linewidth}{!}{
  \begin{tabular}{@{}lccccccc@{}}
    \toprule
    Method                              & Pose2Img              &  TPS       & DreamPose           &    DisCo    & Ours   & Ours w/o TD    & 300 frames w/o TD          \\
    \midrule
    % \multicolumn{7}{l}{Same-domain Motion} \\
    % \midrule
    % Time cost                          &  77s            &  42s           & 610s         &    234s         & 407s         &  301s           & OOM        \\
    Time cost                          &  77s            &  42s           & 310s         &    154s         & 407s         &  301s           & OOM        \\
    Method type                        &  non-diffusion  &  non-diffusion & diffusion    &    diffusion    & diffusion    &  diffusion      & diffusion        \\
    Resolution                         & 640px           &  384px         & 512px        &    256px        & 512px        &  512px          & 512px      \\
    % \midrule
    % \multicolumn{7}{l}{Cross-domain Motion} \\
    % \midrule
    %  w/o TD                             &       48.84       &  18.20          &  344.85        &   1.45            &  4.74         &  5.61              \\
    % w/o FE                              &       40.84       &  16.18          &  124.10        &   1.56           &  -            &   -                \\
    \bottomrule
  \end{tabular}
  }
  % \vspace{-10px}
  \caption{Comparison of time cost to generate 300 frames. }
  \label{tab:ablation.timecost}
  % \vspace{-24px}
\end{table}

\section{High-Resolution FE Model}
% The $22n^{nd}$ second occurs sticking-out-the-tongue, which is an individual habit of the identity.
% Considering how to improve it, we didn't conduct the experiments with 3DMM during the rebuttal period, as SMPL-X (with FLAME for face) and 3DMM represent the face with comparable accuracy as far as we know~[r2].
% The suggestion of replacing SMPL-X with 3DMM is interesting. However, 3DMM only contains facial parameters. Directly utilizing 3DMM may cause inconsistency with SMPL body parameters and increase workload. 
% To improve it, the suggestion of replacing SMPL-X with 3DMM is promising.
% However, we failed to conduct the experiments during the rebuttal period.
% Somtimes 
We observed that our method sometimes generate inaccurate lip and expression movements, this could be dated back to the mouth's small size which constrains face enhancement's ability.
% Otherwise, we found that the mouth's small size constrains face enhancement's ability,
We make a improvement that
% and lip movements can be improved by
training a higher-pixel model from 256px to 512px.
As in Fig.~\ref{fig:512FE} and Table~\ref{tab:512FE}, the lip and expression movements becomes accurate and the quality of the face region is enhanced.
\begin{figure}[htp]
\vspace{-10px}

    \begin{minipage}[t]{0.32\linewidth}
        \includegraphics[width=\linewidth]{gifs/face/000007.png}
    \end{minipage}
    \begin{minipage}[t]{0.32\linewidth}
        \includegraphics[width=\linewidth]{gifs/face/000017.png}
    \end{minipage}
    \begin{minipage}[t]{0.32\linewidth}
        \animategraphics[width=\linewidth,autoplay=True]{15}{gifs/face/0000}{03}{32}
    \end{minipage}
\caption{
    Improved FE. Left 256px, right 512px.
    % For each image, left is pose, and right is output. 
    % The first two images in each subfigure are frames from the video. 
    Click the last image to play the embedded clips with Acrobat Reader.
    % \textit{\small Zoom in for detail. The first two images in each subfigure are frames from the video. Click the last images to play the embedded clips with Acrobat Reader.}
}
% \vspace{-15px}
\label{fig:512FE}
\end{figure}

\begin{table}
  \centering
  \resizebox{.8\linewidth}{!}{
  \begin{tabular}{@{}lcccccc@{}}
    \toprule
    Method                            & FID  &   FVD↓           &    LMD (Face)↓                    \\
    \midrule
    Ours                              & 40.33     &   139.82        &    1.44                   \\
    % Q5 w SMPL perturbation                 &   136.21        &    1.40               &  5.25                 \\
    % Q2 \& Q8 Cross-person motion                   &  145.33        &    1.69          &  5.66                \\
    FE w 512px                        & 39.73     &  140.18        &    1.35                              \\
    % Q11.1 Only train fine-tuning video          &  278.73        &    4.38           &   7.25                \\
    % Q11.2 All train at once                    &  178.79        &    1.56         &   6.01                \\
    % Metrics                              &    Ours   & Q2 \& Q8  & Q5      & Q6     &  Q11.1  & Q11.2 \\
    % \midrule
    %  FVD↓                                &    139.82 & 145.33    & 136.21  & 140.18 &  278.73 & 178.79 \\
    %  LMD (Face)↓                         &    1.44   & 1.69      & 1.40    & 1.35   &  4.38   & 1.56 \\
    %  LMD (Body)↓                         &    4.88   & 4.98      & 4.65    & —     &  5.34   & 4.77 \\
    %  LMD (Hand)↓                         &    5.41   & 5.66      & 5.25    & —      &  7.25   & 6.01 \\
    \bottomrule
  \end{tabular}
  }
  \vspace{-10px}
  \small
  \caption{ Numerical results of FE with 512px.}
  \label{tab:512FE}
  \vspace{-10px}
\end{table}

\section{Liminations}
The generated video results are based on the input 3D mesh sequence. 
When the input mesh sequence is of large pose variations or even inaccurate, the visual quality of the results will be decreased.
As shown in Fig.~\ref{fig:sup.badcase.largepose}, when the driven facial pose largely varies from the training data, the generated facial expressions are unsatisfactory.
It could be improved with more fine-tuning data as shown in Section~\ref{sec:videolength}.
Furthermore, due to limitations in the precision of motion capture, especially regarding the accuracy of hand capture, some obtained motion meshes exhibit inaccuracies.
As shown in Fig.~\ref{fig:sup.badcase.badpsoe}, when the input mesh is inaccurate, the generated frame is confusing.
The inaccurate meshes are reflected in the results, leading to phenomena such as limb misalignment.
% \paragraph{Large Pose Variations.}
% As discussed in Section 7, large poses different from training data may bring unsatisfactory results, as shown in Fig.~\ref{fig:sup.largepose}.
% It could be improved with more fine-tuning data as shown in Section~\ref{sec:videolength}.
% \paragraph{Inaccurate Mesh.}
% Due to limitations in the precision of motion capture, especially regarding the accuracy of hand capture, some obtained motion meshes exhibit inaccuracies. These inaccurate meshes are reflected in the results, leading to phenomena such as limb misalignment.
% An example is given in Fig.~\ref{fig:sup.badcase.badpsoe}.
% \input{figure/large_pose}
% \input{figure/bad_pose}

\begin{figure}[htp]
\newcommand{\galleryfigurewidth}{0.30}
\centering
    %%%%
    \begin{minipage}[t]{\linewidth}
    \centering
        \begin{minipage}{\galleryfigurewidth\linewidth}
            \includegraphics[width=\linewidth]{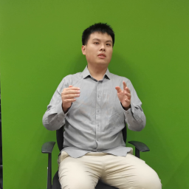}
        \end{minipage}
        \begin{minipage}{\galleryfigurewidth\linewidth}
            \includegraphics[width=\linewidth]{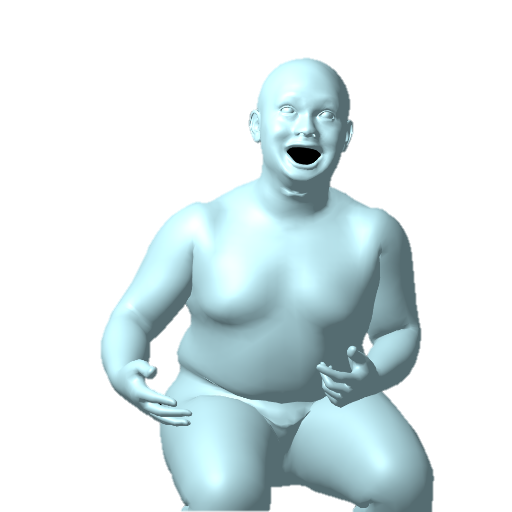}
        \end{minipage}
        \begin{minipage}{\galleryfigurewidth\linewidth}
            \includegraphics[width=\linewidth]{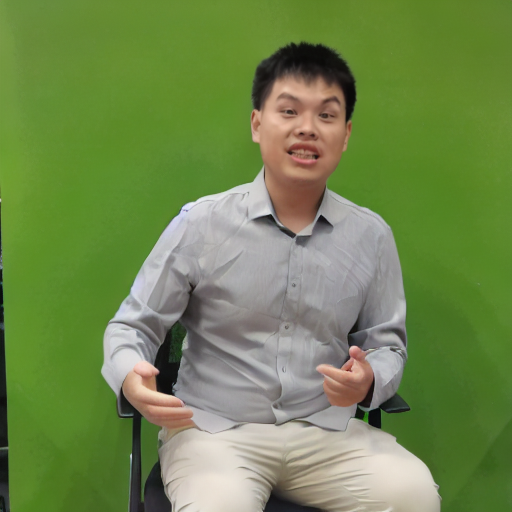}
        \end{minipage}
        \begin{subfigure}[t]{\galleryfigurewidth\linewidth}
                    \subcaption*{Appearance}
        \end{subfigure}
        \begin{subfigure}[t]{\galleryfigurewidth\linewidth}
            \subcaption*{Large pose variation}
        \end{subfigure}
        \begin{subfigure}[t]{\galleryfigurewidth\linewidth}
            \subcaption*{Bad output}
        \end{subfigure}
        \subcaption{}
        \label{fig:sup.badcase.largepose}
    \end{minipage}
    \begin{minipage}[t]{\linewidth}
    \centering
        \begin{minipage}{\galleryfigurewidth\linewidth}
            \includegraphics[width=\linewidth]{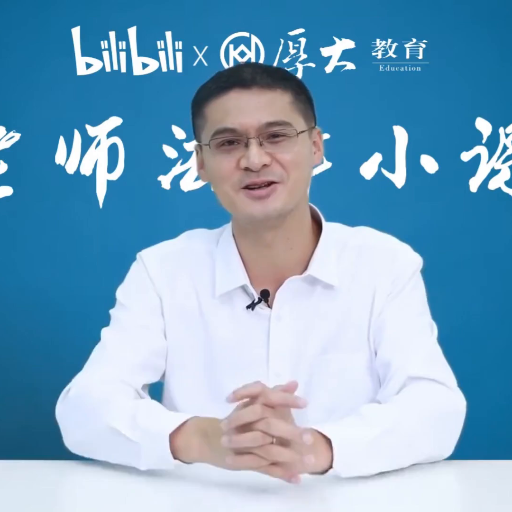}
        \end{minipage}
        \begin{minipage}{\galleryfigurewidth\linewidth}
            \includegraphics[width=\linewidth]{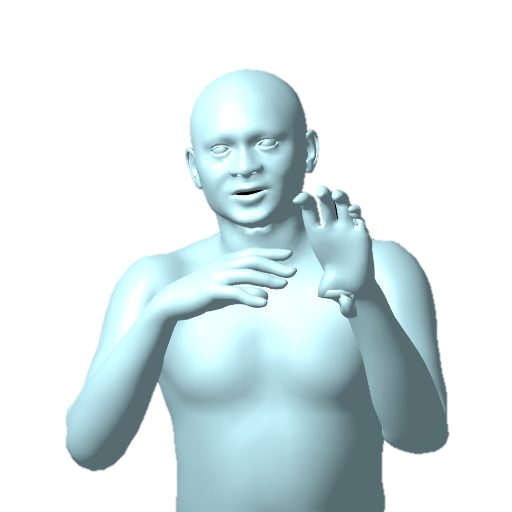}
        \end{minipage}
        \begin{minipage}{\galleryfigurewidth\linewidth}
            \includegraphics[width=\linewidth]{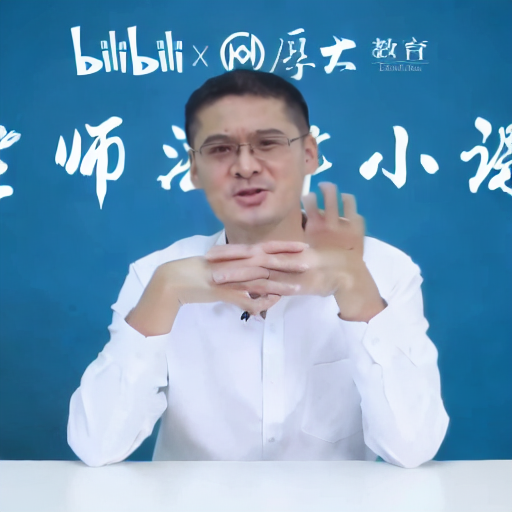}
        \end{minipage}
        \begin{subfigure}[t]{\galleryfigurewidth\linewidth}
            \subcaption*{Appearance}
        \end{subfigure}
        \begin{subfigure}[t]{\galleryfigurewidth\linewidth}
            \subcaption*{Inaccurate pose}
        \end{subfigure}
        \begin{subfigure}[t]{\galleryfigurewidth\linewidth}
            \subcaption*{Bad output}
        \end{subfigure}
        \subcaption{}
        \label{fig:sup.badcase.badpsoe}
    \end{minipage}
\caption{
Limitations. When the driven mesh is of large variation or inaccurate, the generated frame will be unsatisfactory.
}
\label{fig:sup.badcase}
\end{figure}

%\section{Ablation on Overlapped-Batch}

\section{Border Impacts}
Our method could be used maliciously to create DeepFake videos, which may bring adverse social impacts.
% the propagation of fake news.
We deeply understand the possible negative influence of human video generation technology, and will strictly prevent the spread of our method.
Nevertheless, we believe that our approach can yield positive societal impacts, particularly in applications within fields such as education, entertainment, healthcare, and e-commerce.
% Besides, studying the generation methods can help researchers build effective DeepFake detection tools
% ~\cite{}.
% ~\cite{gao2021infoswap, roessler2019ffpp}.
% Apart from the negative usages, there still exists positive applications for human video generation, including entertainment and education.

% {
%     \small
%     \bibliographystyle{ieeenat_fullname}
%     \bibliography{main}
% }

% \label{sec:rationale}
% % 
% Having the supplementary compiled together with the main paper means that:
% % 
% \begin{itemize}
% \item The supplementary can back-reference sections of the main paper, for example, we can refer to \cref{sec:intro};
% \item The main paper can forward reference sub-sections within the supplementary explicitly (e.g. referring to a particular experiment); 
% \item When submitted to arXiv, the supplementary will already included at the end of the paper.
% \end{itemize}
% % 
% To split the supplementary pages from the main paper, you can use \href{https://support.apple.com/en-ca/guide/preview/prvw11793/mac#:~:text=Delete%20a%20page%20from%20a,or%20choose%20Edit%20%3E%20Delete).}{Preview (on macOS)}, \href{https://www.adobe.com/acrobat/how-to/delete-pages-from-pdf.html#:~:text=Choose%20%E2%80%9CTools%E2%80%9D%20%3E%20%E2%80%9COrganize,or%20pages%20from%20the%20file.}{Adobe Acrobat} (on all OSs), as well as \href{https://superuser.com/questions/517986/is-it-possible-to-delete-some-pages-of-a-pdf-document}{command line tools}.
